# Supplementary material for: Incremental Learning with Maximum Entropy Regularization: Rethinking Forgetting and Intransigence
Source: arXiv:1902.00829 source file (2019-02-03)
Supplement: Supplementary file 1 [file 06_appendix.tex]

\section{Appendix}

\section{Datasets}
We evaluate our method on the CIFAR 100~\cite{Krizhevsky09learningmultiple} for the benchmark with many other incremental learning algorithms. 
It consists of 60,000 images with the size of 32$\times$32 pixels in 100 object categories. Among 60,000, 50,000 images are used for training a model and 10,000 images are used for testing. 
We split this dataset into 10 groups of 10 classes for a sequential task similar to \cite{castro2018eccv, Rebuffi_2017_CVPR}.
We evaluate baselines and our method on the CIFAR100 dataset using 1)Densenet121 as the backbone, and 2)Simple 4-Layer CNN as the backbone.
At test of $k^{\text{th}}$ task, the model will be evaluated on a fixed testset composed of classes from all $10 \cdot k$ classes similar to \cite{castro2018eccv, Rebuffi_2017_CVPR}. 
Note that \cite{Chaudhry_2018_ECCV} tests the model only on the 10 new classes but allows the model's confusion to span over all $10 \cdot k$ classes. This difference in task configuration is the primary reason that some of the results show different trends from what was reported by Chaudhry \emph{et. al}. 

We also extend our experiments to the TinyImageNet ~\cite{TinyImageNet} to see how different algorithms work on a bigger dataset.
The TinyImageNet dataset consists of 120,000 images with size of 32 $\times$ 32 pixels in 200 object categories. Of the 120,000 images, 100,000 are used for training, 10,000 for validation, and 10,000 for testing. Note that we opted to use the validation set when testing instead of submitting predicted labels on the testset to the evaluation server held by Standford. 
We have split this dataset into 10 groups of 20 classes similar to our experiment on the CIFAR100 dataset. Therefore, at 
test of $k^{\text{th}}$ task, the model will be evaluated on a fixed testset composed of classes from all $20 \cdot k$ classes it has seen so far.

%\begin{figure}
% \includegraphics[width =\columnwidth]{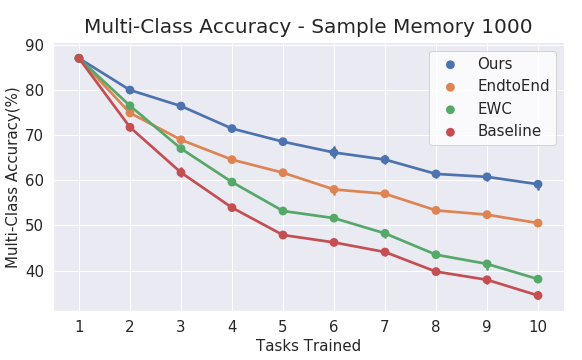}
% \vspace{-8mm}
% \caption{\textbf{Random Curriculum Sample Memory 1000}}
% \label{fig:sample_good}
% \end{figure}

%============================================

================================================
\begin{table*}[!th]
\centering
\resizebox{0.77\paperwidth}{!}{
\begin{tabular}{c|l|l|l|l|l||l|l|l|l}
\hline
      & Unit(\%) & Accuracy $\uparrow$ & A10 $\uparrow$ & F10 $\downarrow$ & I10 $\downarrow$ & SDF10 $\downarrow$ & SDI10 $\downarrow$ & $\text{SDF}_{avg}$ $\downarrow$ & $\text{SDI}_{avg}$ $\downarrow$ \\ \hline\hline
      
    \parbox[t]{2mm}{\multirow{4}{*}{\rotatebox[origin=c]{90}{Rand. Cfg}}} 
      & \ours & \textbf{72.51$\pm$0.17} &  \textbf{73.35$\pm$0.35} &  \textbf{0.13$\pm$0.16} &  \textbf{9.68$\pm$0.44} &  \textbf{5.05$\pm$0.10} &  \textbf{13.14$\pm$0.28} &  \textbf{2.96$\pm$0.06} &  \textbf{6.55$\pm$0.26}
      \\ \cline{2-10}
      & EndtoEnd & 66.56$\pm$0.05 &  63.46$\pm$0.22 &  3.52$\pm$0.31 &  18.80$\pm$0.39 &  6.79$\pm$0.19 &  24.58$\pm$0.29 &  3.90$\pm$0.09 &  11.72$\pm$0.06 \\ \cline{2-10}
      & EWC & 64.75$\pm$0.14 &  65.70$\pm$0.37 &  1.36$\pm$0.41 &  24.18$\pm$0.23 &  9.68$\pm$0.31 &  18.10$\pm$0.69 &  5.98$\pm$0.07 &  7.71$\pm$0.15 \\ \cline{2-10}
      & Baseline & 62.64$\pm$0.26 &  64.40$\pm$0.29 &  0.21$\pm$0.32 &  25.01$\pm$0.33 &  10.17$\pm$0.36 &  18.80$\pm$0.31 &  6.49$\pm$0.10 &  8.42$\pm$0.11 \\ \hline%\cline{2-10}
      & Reference & 77.85$\pm$0.00 &  80.21$\pm$0.00 &  0.58$\pm$0.00 &  -0.03$\pm$0.00 &  0.00$\pm$0.00 &  0.00$\pm$0.00 &  1.40$\pm$0.00 &  3.20$\pm$0.00 \\ 
      \hline

    \parbox[t]{2mm}{\multirow{4}{*}{\rotatebox[origin=c]{90}{Best Cfg}}} 
      & \ours & \textbf{83.80$\pm$0.14} &  \textbf{84.28$\pm$0.06} &  \textbf{0.48$\pm$0.03} &  \textbf{2.56$\pm$0.24} &  \textbf{2.14$\pm$0.02} &  \textbf{12.11$\pm$0.44} &  \textbf{1.15$\pm$0.03} &  \textbf{4.57$\pm$0.05} \\ \cline{2-10}
      & EndtoEnd & 82.16$\pm$0.08 &  82.34$\pm$0.26 &  0.75$\pm$0.15 &  5.45$\pm$0.40 &  2.27$\pm$0.11 &  16.09$\pm$0.39 &  1.18$\pm$0.01 &  6.19$\pm$0.14 \\ \cline{2-10}
      & EWC & 72.70$\pm$0.17 &  72.44$\pm$0.35 &  2.46$\pm$0.39 &  22.65$\pm$0.56 &  7.35$\pm$0.14 &  18.83$\pm$0.71 &  4.11$\pm$0.05 &  6.62$\pm$0.14 \\ \cline{2-10}
      & Baseline & 70.24$\pm$0.20 &  71.06$\pm$0.09 &  1.48$\pm$0.15 &  25.45$\pm$0.21 &  8.18$\pm$0.23 &  19.37$\pm$0.58 &  4.72$\pm$0.02 &  7.14$\pm$0.12 \\ \hline % \cline{2-10}
      & Reference & 84.44$\pm$0.00 & 85.77$\pm$0.00 & 0.07$\pm$0.00 & 0.00$\pm$0.00 &  0.00$\pm$0.00 & 0.00$\pm$0.00 & 0.77$\pm$0.00 & 2.33$\pm$0.00 \\ \hline
      \hline
      
    \parbox[t]{2mm}{\multirow{4}{*}{\rotatebox[origin=c]{90}{Worst Cfg}}} 
      & \ours & \textbf{63.33$\pm$0.18} &  \textbf{65.21$\pm$0.20} &  \textbf{0.16$\pm$0.22} &  \textbf{5.11$\pm$0.19} &  \textbf{5.12$\pm$0.05} &  \textbf{10.54$\pm$0.26} &  \textbf{3.79$\pm$0.10} &  \textbf{6.92$\pm$0.09}
 \\ \cline{2-10}
      & EndtoEnd & 55.86$\pm$0.06 &  57.44$\pm$0.39 &  0.43$\pm$0.37 &  14.39$\pm$0.04 &  7.40$\pm$0.17 &  14.80$\pm$0.34 &  5.57$\pm$0.10 &  8.89$\pm$0.10 \\ \cline{2-10}
      & EWC & 50.52$\pm$0.32 &  49.85$\pm$0.25 &  2.51$\pm$0.06 &  24.55$\pm$0.43 &  10.41$\pm$0.35 &  19.18$\pm$0.19 &  8.33$\pm$0.09 &  9.38$\pm$0.10 \\ \cline{2-10}
      & Baseline & 44.72$\pm$0.27 &  46.25$\pm$0.50 &  0.58$\pm$0.74 &  29.43$\pm$0.26 &  12.19$\pm$0.27 &  22.73$\pm$0.33 &  10.75$\pm$0.18 &  11.06$\pm$0.10 \\ \hline% \cline{2-10}
      & Reference & 67.52$\pm$0.00 &  71.28$\pm$0.00 &  -0.38$\pm$0.00 &  0.00$\pm$0.00 &  0.00$\pm$0.00 &  0.00$\pm$0.00 &  2.12$\pm$0.00 &  3.45$\pm$0.00 \\ \hline
      
\end{tabular}}
\caption{\textbf{Incremental Learning Performance with Reference} `Rand. Cfg' refers to random task configurations, `Best Cfg' refers to the best first task configuration (See text in Sec.\ref{}), `Worst Cfg' refers to the worst first task configuration (See text in Sec.\ref{}). $\uparrow$ indicates higher number is better, $\downarrow$ otherwise. Accuracy is averaged multi-class accuracy from task 1 to task 10. Numbers after $\pm$ denotes standard deviation. Results on the eight metrics for methods tested on the Random configuration using the CIFAR100 dataset. Best results are in bold for each of the eight metrics. EWC is elastic weight consolidation by \cite{Kirkpatrick2017OvercomingCF} and EndtoEnd is End to End incremental learning by \cite{castro2018eccv}.}
\label{table:alpha_curi_with_ref}
\end{table*}

\subsection{Qualitative Analysis}

\paragraph{Classwise Accuracy Tracking.} 
We show the classwise accuracy of the first task as the incremental learning goes on. Note that all 10 classes show a general drop in accuracy to varying extent. Across all classes, EWC and the Baseline show jagged changes in the classwise accuracy more often than \ours~or EndtoEnd. In Figure \ref{fig:apples}
% \jb{The figure citation and the real figure index that appears on the paper does not match. Is it okay?}\dk{yes, it's one of the great things about latex}
, one can see that EWC and the Baseline experience sharply drops in accuracy at task 6 and task 9. Similar drops in accuracy is observed in other plots as well. Although the general drop in accuracy is observed for all methods across the 10 classes, some classes show considerably different behavior for different methods. For example, in figure \ref{fig:bee}, \ours~retain a considerably higher accuracy from task 2 to task 10 and show less degradation in accuracy \jb{how about showing the ratio of degradation} compared to the other methods. In addition, \ours~displays a smoother decline in classwise accuracy for most of the 10 classes, indicating that it is more robust to catastrophic forgetting.

% \begin{figure}
% \centering
% \includegraphics[width=0.80\columnwidth]{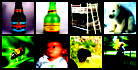}
% \caption{\textbf{Samples used in Sample Tracking}}
% \label{fig:sample_update}
% \end{figure}

\begin{figure}
\includegraphics[width =\columnwidth]{images/apples_acc_track(UPDATE).png}
\vspace{-8mm}
\caption{\textbf{Classwise Acc- Apples}}
\label{fig:apples}
\end{figure}

\begin{figure}
\includegraphics[width =\columnwidth]{images/aquarium_fish_acc_track(UPDATE).png}
\vspace{-8mm}
\caption{\textbf{Classwise Acc - Aquarium Fish}} 
\label{fig:aqfish}
\end{figure}

\begin{figure}
\includegraphics[width =\columnwidth]{images/baby_acc_track(UPDATE).png}
\vspace{-8mm}
\caption{\textbf{Classwise Acc - Baby}}
\label{fig:baby}
\end{figure}

\begin{figure}
\includegraphics[width =\columnwidth]{images/bear_acc_track(UPDATE).png}
\vspace{-8mm}
\caption{\textbf{Classwise Acc - Bear}}
\label{fig:bear}
\end{figure}

\begin{figure}
\includegraphics[width =\columnwidth]{images/beaver_acc_track(UPDATE).png}
\vspace{-8mm}
\caption{\textbf{Classwise Acc - Beaver}}
\label{fig:beaver}
\end{figure}

\begin{figure}
\includegraphics[width =\columnwidth]{images/bed_acc_track(UPDATE).png}
\vspace{-8mm}
\caption{\textbf{Classwise Acc - Bed}}
\label{fig:bed}
\end{figure}

\begin{figure}
\includegraphics[width =\columnwidth]{images/bee_acc_track(UPDATE).png}
\vspace{-8mm}
\caption{\textbf{Classwise Acc - Bee}}
\label{fig:bee}
\end{figure}

\begin{figure}
\includegraphics[width =\columnwidth]{images/beetle_acc_track(UPDATE).png}
\vspace{-8mm}
\caption{\textbf{Classwise Acc - Beetle}}
\label{fig:beetle}
\end{figure}

\begin{figure}
\includegraphics[width =\columnwidth]{images/bicycle_acc_track(UPDATE).png}
\vspace{-8mm}
\caption{\textbf{Classwise Acc - Bicycle}}
\label{fig:bicycle}
\end{figure}

\begin{figure}
\includegraphics[width =\columnwidth]{images/bottles_acc_track(UPDATE).png}
\vspace{-8mm}
\caption{\textbf{Classwise Acc - Bottles}}
\label{fig:bottles}
\end{figure}

\paragraph{Sample Tracking.} 
From the first task to the final task, we identify four scenarios of changing classification confidence of each sample given in the first task; 1) high to high, 2) high to low, 3) low to high and 4) low to low. For each scenario, we randomly choose two samples per scenario  and track and plot the confidence of them as task progresses in Figure~\ref{fig:sample_good} and \ref{fig:sample_bad}.
% delete (so eight samples shown in Figure \ref{fig:sample_update})
% We show eight samples from the first task and plot their respective confidence as our model progresses through the incremental learning setting.

% In Figure \ref{fig:sample_update}, we show images of the samples that were tracked. 
% The top row corresponds to the samples used in Fig \ref{fig:sample_good} where we track samples that originally had high confidence, and the bottom row corresponds to the samples with low confidence used in Fig \ref{fig:sample_bad}. 

\begin{figure}
\includegraphics[width =\columnwidth]{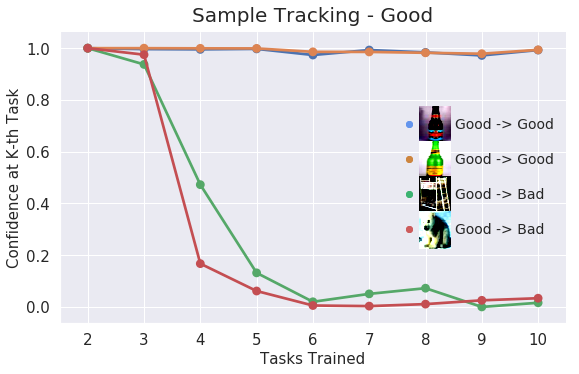}
\vspace{-8mm}
\caption{\textbf{Sample Tracking-Good}}
\label{fig:sample_good}
\end{figure}

In figure \ref{fig:sample_good}, we see two very distinct groups where two samples retain their high confidence throughout the incremental learning process while the other two samples' confidence drops dramatically at around task 3 - 4. 
This is an example of catastrophic forgetting, showing that even samples that were classified with very high confidence can be forgotten as the stream of tasks go on.

In contrast, we see two interesting cases of samples that originally has low confidence but has high confidence at the final task, shown in Figure \ref{fig:sample_bad}. 
% Some samples actually increase in confidence as the tasks progress, reaching over 0.8 by the end of the incremental learning setting. 
% Given, that these samples originally started out with under 0.2 confidence, it shows the case in which incremental addition of classes actually help in classifying a given sample. 
% Furthermore, we see two samples whose originally low confidence reach the maximum confidence at task 4 but gradually reduces to a low level close to its original value. 
You can see that the first sample in the bottom row of figure \ref{fig:sample_update} can be easily confused to be in the 'Beetles' class while it is in the 'Bee' class. 
Similarly, the second sample in the bottom row of figure \ref{fig:sample_update} shows an image of a baby with a red face, easily mistaken to be a sample of 'Apples' class. As the tasks progress, the newly added classes such as 'Lawn Mower', 'Lamp', 'Leopard', and 'Mountain' in task 5 serve as easy negatives, increasing the confidence of the two samples. 

The last two samples in the bottom row of figure \ref{fig:sample_update} enjoy a temporary increase in confidence at task 4, their confidence drops to near zero in the final task. 
While addition of easy negatives can contribute to the increase in confidence for some samples, the increase does not always last.

\begin{figure}
\includegraphics[width =\columnwidth]{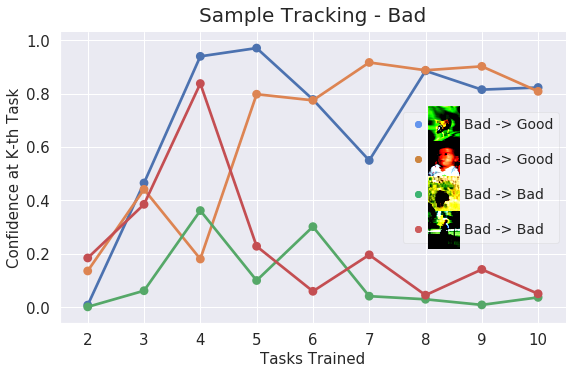}
\vspace{-8mm}
\caption{\textbf{Sample Tracking-Bad}}
\label{fig:sample_bad}
\end{figure}

\subsection{Experiments on TinyImageNet}

\begin{figure}[h!]
\centering
\includegraphics[width=1\columnwidth]{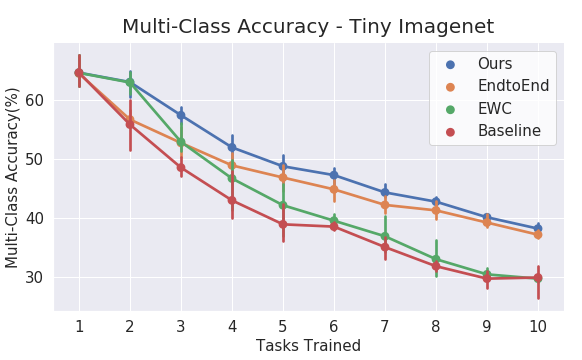}
\vspace{-8mm}
\caption{\textbf{Multi-Class Accuracy - TinyImageNet.} Plots are reported with error bars from 3 trials.}\label{fig:timage}
\end{figure}

% \begin{table*}[!th]
% \centering
% \resizebox{0.77\paperwidth}{!}{
% \begin{tabular}{l|l|l|l|l||l|l|l|l}
% \hline
% Methods & Accuracy $\uparrow$ & A10 $\uparrow$ & F10 $\downarrow$ & I10 $\downarrow$ & SDF10 $\downarrow$ & SDI10 $\downarrow$ & $\text{SDI}_{avg}$ $\downarrow$ & $\text{SDI}_{avg}$ $\downarrow$ \\ \hline
% \ours &  0.899$\pm$0.0044& 0.875$\pm$0.0075 & 0.029$\pm$0.0142 & 0.115$\pm$0.0102 & 0.267$\pm$0.0567 & 0.313$\pm$0.1128 & 0.146$\pm$0.0033 & 0.148$\pm$0.0634 \\ \hline
% EndtoEnd  & - & - & - & - & - & - & - & - \\ \hline
% EWC  & 0.887$\pm$0.019 & 0.900$\pm$0.013 & -0.021$\pm$0.0074 & 0.139$\pm$0.032 & 0.026$\pm$0.0233 & 0.979$\pm$0.0064 & 0.053$\pm$0.0156 & 0.027$\pm$0.0082 \\ \hline
% Baseline  & 0.840$\pm$0.0027 & 0.869$\pm$0.0043 & -0.019$\pm$0.0076 & 0.208$\pm$0.0239 & 0.240$\pm$0.0198 & 0.217$\pm$0.0961 & 0.146$\pm$0.0154 & 0.131$\pm$0.0498 \\ \hline
% \end{tabular}}
% \caption{\textbf{FashionMNIST Random Curriculum.}}\label{table:table5}
% \end{table*}
